# Supplementary material for: On the convergence of Hamiltonian Monte Carlo
Source: arXiv:1705.00166 source file (2019-05-10)
Supplement: Supplementary file 1 [file appendix.tex]

% \begin{assumption}[$\expozero$]
%   \label{assum:regOne_alt}
%   $F$ is continuously differentiable and there exist $\constzero, \constzeroD \geq 0$ and $\expozero \in \ccint{0,1}$ such that for all $x,y \in \rset^d$ 
% \begin{equation*}
% \abs{\nabla F(x) - \nabla F(y)} \leq \constzero \min \parenthese{\abs{x-y}, \abs{x-y}^\expozero + \constzeroD} \eqsp.    
%   \end{equation*}
% \end{assumption}

% \begin{lemma}
%   \label{lem:app_eq_assum_0}
%   \Cref{assum:regOne}$(\expozero)$ and \Cref{assum:regOne_alt}$(\expozero)$ are equivalent.
% \end{lemma}

% \begin{proof}
%   It is straightforward that \Cref{assum:regOne}  implies   \Cref{assum:regOne_alt}. The converse just comes from the fact that for all $R \geq 0$,  $x,y\in \rset^d$, $\abs{x-y} \leq R$,
% \begin{equation*}
%     \abs{\nabla F(x) - \nabla F(y)} \leq \constzero R^{1-\expozero} \abs{x-y}^{\expozero} \eqsp,
%   \end{equation*}
% and for all $x,y\in \rset^d$, $\abs{x-y} \leq \constzeroD^{1/\expozero}$,
% \begin{equation*}
%     \abs{\nabla F(x) - \nabla F(y)} \leq 2 \constzero  \abs{x-y}^{\expozero} \eqsp.
%   \end{equation*}
% Therefore \Cref{assum:regOne_alt} implies \Cref{assum:regOne} with $\constzero \leftarrow  (\constzero \constzeroD^{(1-\expozero)/\expozero}) \vee (2 \constzero) $. 
% \end{proof}

% \begin{lemma}
%   \label{lem:1}
%   \begin{enumerate}
%   \item $\{\Phiverlet[h][T]\}^{-1}(q,p) = \Phiverlet[h][T](q,-p)$

%   \end{enumerate}
% \end{lemma}

%%% Local Variables: 
%%% mode: latex
%%% TeX-master: "main"
%%% End: 
